# Supplementary material for: Pedestrian Emergence Estimation and Occlusion-Aware Risk Assessment for Urban Autonomous Driving
Source: arXiv:2107.02326 source file (2021-07-06)
Supplement: Supplementary file 1 [file appendix2.tex]

\label{sec:risk_zones}
Since the ego vehicle is not in control of the location and velocity of pedestrians, the main factor for driving safety is related to \eqref{eq:collision_distcond_2}. As one can see, there are two variables that the ego vehicle cannot control, but only measure or estimate: $t_{sense}$ and $t_{system\_delay}$; whereas there are three variables that the ego vehicle can control within their physical limits: $v_{ego}$, $a_f$, and $t_{ramp}$.

\begin{gather}
    \frac{2d_p - w_{ego}}{2v_{ped}} \leq \frac{2d_o}{2v_{ego}} \leq \frac{2d_p + w_{ego}}{2v_{ped}}\label{eq:collision_timecond_2}\\
    \begin{split}
        d_o &\leq d_{stop}\\
        &= \frac{v_{ego}^2}{2a_f} + \frac{v_{ego} t_{ramp}}{2} - \frac{a_{f} t_{ramp}^2}{24}\\
        &+ v_{ego} * ( t_{sense} + t_{system\_delay})\\
        &+ d_{safe}
    \end{split}\label{eq:collision_distcond_2}
\end{gather}

One can categorize the control of these variables in three aspects: \textit{comfort, safety}, and \textit{efficiency}. A successful policy can be considered as the one which optimizes these three aspects together, ideally for all road users whom the vehicle interacts. Let us denote the positive value for maximum deceleration of the ego vehicle as $a_{max}$ and the minimum possible time to reach a steady acceleration/deceleration value as $t_{ramp\_min}$, and the maximum velocity that ego vehicle is legally allowed to drive as $v_{ego\_max}$. Let us also assume that these values are constant. Provided that the ego vehicle is in a situation in which it is required to ensure safety, it is assumed that the ego vehicle will try to reach the steady deceleration of $a_{max}$ with its limiting time $t_{ramp\_min}$, let us assume that under this policy the earliest distance that the ego vehicle can stop is $d_{stop\_min}$. On the other hand, when there is no indication of danger, it is assumed that the ego vehicle will try to reach $v_{ego\_max}$. 

To define an optimal policy in terms of comfort, one should start from what a passenger inside a car feels and how the feeling of comfort is affected. Human passengers can merely guess the speed of the vehicle with other visible objects from other frame of references, such as a standing car passed by; however, a passenger can in fact feel both the force, and the change in force applied to their bodies which is also known as \textit{jerk}. Since both acceleration and jerk perceived by the human body omni-directionally, one can define a $a_{comfort}$, and a $j_{comfort}$ value which it can be assumed that an acceleration between $[-a_{comfort}, a_{comfort}]$ values and a jerk between $[-j_{comfort}, j_{comfort}]$ are considered to be \textit{comfortable}. Let us denote the distance that the ego vehicle can stop when its positive value of deceleration as $a_{comfort}$ and the time to reach this deceleration value within \textit{comfort} zone as $t_{ramp\_comfort}$. Let us assume that under this policy the earliest distance that the ego vehicle can stop is $d_{stop\_comfort}$.

Using the aforementioned terminology, the ego vehicle can be considered to have imaginary zones, so-called \textit{risk zones} as in Fig.~\ref{fig:zones}. 

Assuming that $d_{stop\_min} \leq d_{stop\_comfort}$, and a reference frame whose origin is at the CoG of the frontal structure of the ego vehicle is used to define the \textit{risk zones}, the longitudinal ranges of the zones are as follows:
\begin{itemize}
    \item Danger Zone : $[0, d_{stop\_min}]$
    \item Discomfort Zone : $[d_{stop\_min}, d_{stop\_comfort}]$
    \item Safety Zone : $[d_{stop\_comfort}, r_{visible}]$
\end{itemize}

Note that for different driving speeds, these three zones may submerge and these are in fact the key factor to determine the risk. For example, given a scenario as demonstrated in fig.~\ref{fig:zones}, the ego vehicle can actually avoid a collision with all of the pedestrians except the one closest to the vehicle if they were to start crossing and their future trajectory enters the expected path of the ego vehicle. Therefore, if it were possible for the closest pedestrian to reach the middle lane before the ego vehicle, the ego vehicle would be jeopardizing the safety of the passengers and VRUs.  

\begin{figure}[t]
     \centering
     \includegraphics[width=\linewidth]{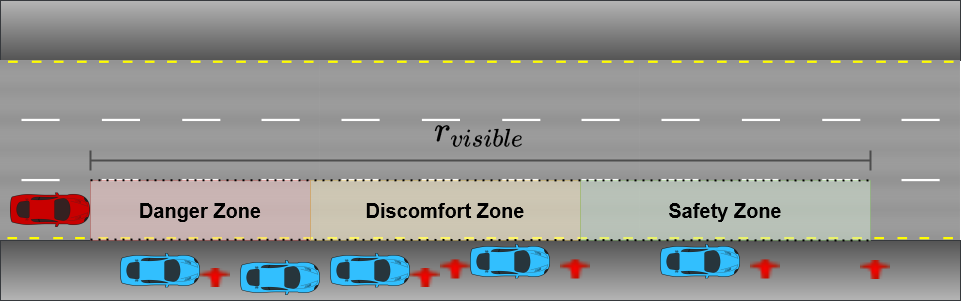}
     \caption{Given the limitations of the ego vehicle, the ego vehicle can \textit{safely} and \textit{comfortably} yield to any pedestrians crossing inside the \textit{Safety Zone}, whereas the ego vehicle is required to compromise on the passengers' \textit{comfort} in order to yield to the pedestrians inside the \textit{Discomfort Zone}. Finally it is not possible to yield or stop before hitting to a pedestrian inside the \textit{Danger Zone} (Zone sizes are not to scale)}
     \label{fig:zones}
\end{figure}
