# Supplementary material for: Pedestrian Emergence Estimation and Occlusion-Aware Risk Assessment for Urban Autonomous Driving
Source: arXiv:2107.02326 source file (2021-07-06)
Supplement: Supplementary file 2 [file appendix3.tex]

The parameters used the simulation, and the scenarios used to evaluate the proposed method against the baselines are provided in Table~\ref{tab:sim_params}~and~\ref{tab:sim_events}.

\begin{table}[h!]
\centering
\caption{Parameters used in the Simulation Environment}
\label{tab:sim_params}
\resizebox{\linewidth}{!}{%
\begin{tabular}{@{}lcr@{}}
\toprule
\textbf{Parameters} & \textbf{Symbol} & \textbf{Values} \\
\midrule
Road length & $l_{road}$ & 96 $m$\\
Lane width & $w_{lane}$ & 3 $m$\\
Number of lanes & N/A & 3\\
Simulation window size & N/A & 1920$\times$550 pixels\\
Pedestrian dimensions & $(l_{ped}\times w_{ped})$ & $(0.5 \times 0.6)$ $m$ (\cite{schram2015euro})\\
Car dimensions & $(l_{car} \times w_{car})$ & $(4 \times 1.75)$ $m$\\
Simulation pixel per meter & N/A & 20 $pixels/m$\\
Maximum possible jerk & $jerk_{max}$ & 28.5714 $m/s^3$ (\cite{edwards_nathanson_wisch_2014})\\
Minimum possible deceleration & $a_{min}$ & $-g * \mu_{road}$ $m/s^2$\\
Maximum possible acceleration & $a_{max}$ & 2 $m/s^2$ \\
Road length & $l_{road}$ & 96 m \\
Maximum visible distance for ego vehicle & $d_{visible}$ & 50 m \\
Pedestrian speed & $v_{pedestrian}$ & 5 km/h \\
Angle of view & $\theta_{view}$ & $[-60^{\circ}, 60^{\circ}]$ \\
\bottomrule
\end{tabular}
}
\end{table}

\begin{table}[h!]
\centering
\caption{Scenarios used in the Simulation Environment}
\label{tab:sim_events}
\resizebox{\linewidth}{!}{%
\begin{tabular}{@{}cllr@{}}
\toprule
\textbf{Scenario} & \textbf{Road Type} & \textbf{Number of parked cars} & \textbf{Crosswalk} \\ \midrule
Suburban scenario (Scenario 1) & Straight Road & Several (At most 2) & Yes\\ 
Mildly crowded street (Scenario 2) & Straight Road & Multiple, all parking slots are full & Yes\\ 
Very crowded street (Scenario 3) & Straight Road & Multiple, but not all parking slots are full & Yes\\ \bottomrule
\end{tabular}
}
\end{table}
