# Supplementary material for: Pedestrian Emergence Estimation and Occlusion-Aware Risk Assessment for Urban Autonomous Driving
Source: arXiv:2107.02326 source file (2021-07-06)
Supplement: Supplementary file 3 [file appendix4.tex]

A collision occurs when a dynamic obstacle reaches a point inside the object's expected path, the object coincides with the obstacle before the obstacle could depart from the expected path. Of course, one can notice that there is another way for a collision to occur, which is when an obstacle coincides with the object from the object's sides; however, that kind of collision is not going to be considered in this thesis since it is collision in which the object is free of blame (use citation of blame notion) 
    
Therefore, the object can collide with an obstacle either: 
\begin{itemize}
    \item is already inside the expected path, and is to stay on the path,
    \item or the obstacle can be outside of the expected path, and is to enter the expected before the object arrives.
\end{itemize}  

For a static obstacle which is waiting ahead, the object's limitation is its visibility range, $r_{visible}$. Due to vehicle's physical limitation, $t_{ramp}$ seconds are required to reach a steady deceleration:
For $t \in [0, t_{ramp}]$:

\begin{align}
     a(t) &= \frac{a_f*t}{t_{ramp}}\label{eq:acc}\\
     v(t) &= \int_0^t a(t) dt + v_0 = v_0 - \frac{a_f * t^2}{2t}\label{eq:velocity}\\
     \begin{split}
         d(t) &= \int_0^t v(t) dt + v_0 * t\\
         &= v_0*t - \frac{a_f * t^3}{6t}
     \end{split}\label{eq:distance}
\end{align}
Then, at $t = t_{ramp}$:
\begin{gather}
     v_{ramp} = v_0 - \frac{a_f * t_{ramp}}{2}\label{eq:v_ramp}\\
     d_{ramp} = v_0 * t_{ramp} - \frac{a_f*t_{ramp}}{6}\label{eq:d_ramp}\\
     d_{steady\_deceleration} = \frac{v_{ramp}^2}{2a_{f}}\label{eq:d_steady}
\end{gather}
Then, total distance the object travels before stopping from the instance of actuating brakes:
\begin{equation}
     \begin{split}
         d_{stop}' &= d_{ramp} + d_{steady\_deceleration}\\
         &= \left (v_0*t_{ramp} - \frac{a_f*t_{ramp}^2}{6} \right)\\
         &+ \left( \frac{v_0^2}{2*a_f} + \frac{a_f*t_{ramp}^2}{8} \right .\\
         &- \left . \frac{v_0*t_{ramp}}{2} \right)\\
         &= \frac{v_0^2}{2a_f} + \frac{v_0 t_{ramp}}{2} - \frac{a_{f} t_{ramp}^2}{24}
     \end{split}
     \label{eq:d_stop1}
\end{equation}

Finally, including the time to sense obstacles, $t_{sense}$, and the time to actuate the brakes, $t_{system\_delay}$, the total distance that the object travels before stopping is:
\begin{equation}
     \begin{split}
         d_{stop} &= d_{ramp} + d_{steady\_deceleration} + d_{delays}\\
         &= \frac{v_0^2}{2a_f} + \frac{v_0 t_{ramp}}{2} - \frac{a_{f} t_{ramp}^2}{24}\\
         &+ v_0 * ( t_{sense} + t_{system\_delay})
     \end{split}
     \label{eq:d_stop2}
\end{equation}

Note that, $a_f$ is a positive acceleration value which is the absolute value of the steady braking deceleration of the object. The object should always ensure that $r_{visible} > d_{stop}$.

Assuming the point mass model for the vehicle, the maximum deceleration value which is possible can be written as:
\begin{equation}
    a_{max} = \mu_{road} *  g
    \label{eq:maximum_decel}
\end{equation}
where $\mu_{road}$ is the road friction coefficient, and $g$ is the gravitational acceleration value. However, as one can expect, the road friction coefficient varies with different weather conditions and road material. \cite{wallman2001friction} gathered the variations due to weather conditions, which is listed in Table~\ref{table:friccoeff_diffweather}.

Assuming that one can obtain the road friction coefficient, either by measuring it or estimating it from the road conditions, and that one can calculate $a_{max}$, then one can also calculate $d_{stop}$ value from \eqref{eq:d_stop2}. However, there is also another variable necessary in order to calculate $d_{stop}$, which is $t_{ramp}$. It is a challenging task to actually obtain limitation for a vehicle, and it is different for different vehicles. However, one can use the AEB standards for $t_{ramp}$ as in a situation in which the maximum braking is required, the AEB system is going to be activated. One can see Appendix to see the conditions required for the activation of AEB systems. \cite{edwards_nathanson_wisch_2014} provided a typical $t_{ramp}$ value in AEB systems for 2018+ generation vehicles to be 0.35 secs.

$d_{stop}$ for $a_{max}$ should always be strictly smaller than visible range $r_{visible}$, that is, the vehicle should never drive a velocity that results in a $d_{stop}$ value greater than $r_{visible}$. For the comfortable driving, \cite{bae2020self} provided values for both acceleration and jerk values.

\begin{table}[h!]
\centering
\caption{Value range for the road friction coefficient for different weather conditions (taken from \cite{wallman2001friction})}
\label{table:friccoeff_diffweather}
\resizebox{0.7\linewidth}{!}{%
\begin{tabular}{@{}lc@{}}
\toprule
\textbf{Condition}     & \textbf{Value Range}              \\ \midrule
Dry bare surface       & [0.80, 1.0]                     \\
Wet bare surface  & [0.70, 0.80] \\
Loose snow & [0.20, 0.50] \\
Packed snow & [0.20, 0.30] \\
Black ice & [0.15 0.30]\\
Loose snow on black ice & [0.15, 0.25]\\
Wet black ice & [0.05, 0.10]\\ \bottomrule
\end{tabular}
}
\end{table}
